# Supplementary material for: Gyrokinetic Simulations for Spherical Tokamak Divertor Design
Source: arXiv:2605.22960 source file (2026-05-21)
Supplement: Supplementary file 1 [file appendix-geo-consistency.tex]

\chapter{Geometric Consistency for Advection Equations}
\label{sec:appendix}

Consider the advection equation
\begin{align}
  \pfrac{f}{t} + \nabla\cdot(\mvec{v} f) = 0 \label{eq:advect}
\end{align}
where $\mvec{v}(\mvec{x},t)$ is a specified velocity profile, and
$f(\mvec{x},t)$ is a scalar advected quantity. We wish to solve this
equation on a non-rectangular domain, including on domains that can't
be covered by a single coordinate patch.

For this introduce computational coordinates $(z^1,z^2,z^3)$ and the
mapping from computational to physical space, as described in the main
text, using $\mvec{x} = \mvec{x}(z^1,z^2,z^3)$. Transforming the
advection equation to this new coordinate system we get
\begin{align}
  \pfrac{f}{t} 
  + \frac{1}{J_c}\pfraca{z^i}\left(J_c \dbasis{i}\cdot\mvec{v} f \right) 
  = 
  0. \label{eq:advect-cs}
\end{align}
In this equation now $f = f(z^i,t)$. 
\begin{figure}
  \incfig{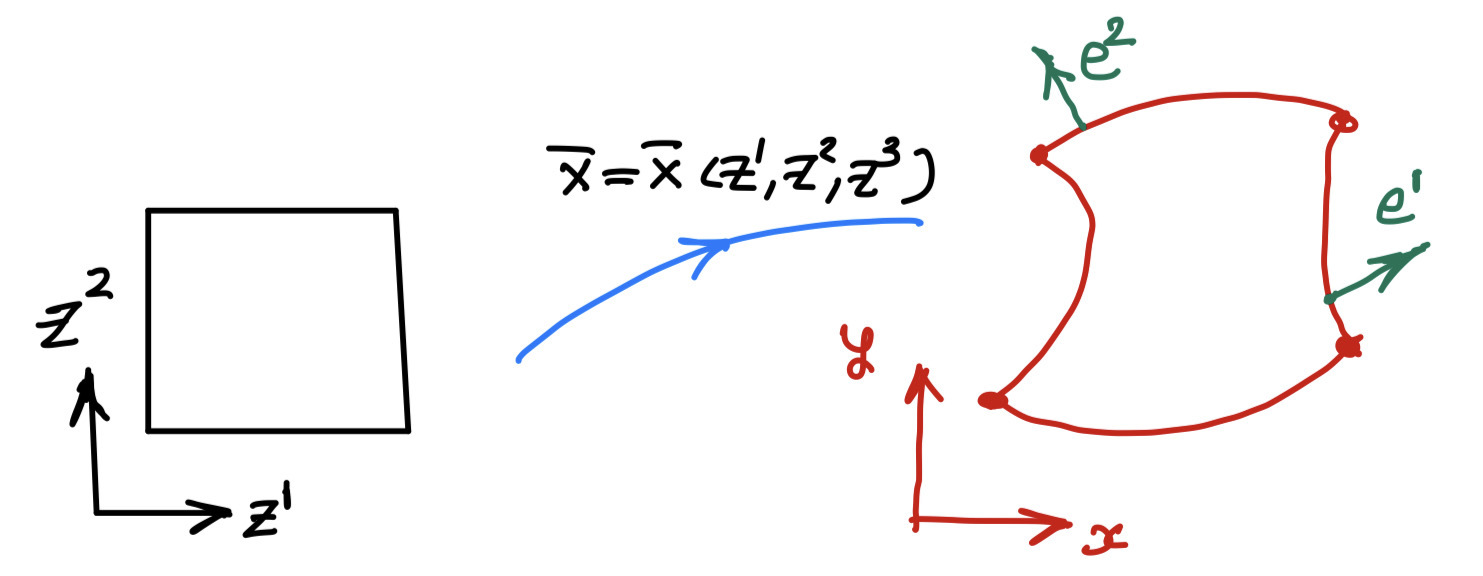}
  \caption{The mapping $\mvec{x} = \mvec{x}(z^1,z^2,z^3)$ maps a
    rectangle in computational space to a region in physical
    space. All information needed to compute the various geometric
    quantities in physical space (volumes, surface-areas, etc) are
    contained in the mapping function. The tangent vectors $\basis{i}$
    are tangent, and dual vectors $\dbasis{i}$ are normal, to the
    mapped faces.}
  \label{fig:mapc2p}
\end{figure}

Now consider a rectangular region in computational space. In general,
this will be mapped to a non-rectangular region in physical space. See
Fig.\thinspace(\ref{fig:mapc2p}). The volume of the mapped region is
\begin{align}
  \mathcal{V} = \iiint J_c \thinspace dz^1dz^2 dz^3.
\end{align}
In this expression we see the appearance of the ``volume element'' in
computational space $dz^1dz^2 dz^3$. This \emph{need not} have the
units of volume in physical space. However, the quantity
$J_c \thinspace dz^1dz^2 dz^3$ \emph{does} have the units of volume
(i.e length cubed).

The surface area of a face, for example, the surface that corresponds
to $z^1 = \textrm{constant}$, can be computed from
\begin{align}
  \mathcal{S}_1 
  =
  \iint \| \dbasis{1} \| J_c \thinspace dz^2 dz^3
  =
  \iint \| \basis{2}\times\basis{3} \| \thinspace dz^2 dz^3.
\end{align}
Hence, we can interpret $\| \dbasis{1} \| J_c$ or
$\| \basis{2}\times\basis{3} \|$ as the \emph{surface Jacobian} for
the $z^1 = \textrm{constant}$ face. The computational space ``surface
element'' $dz^2 dz^3$ \emph{need not} have the units of area in
physical space, but of course
$\| \dbasis{1} \| J_c \thinspace dz^2 dz^3 = \|
\basis{2}\times\basis{3} \| \thinspace dz^2 dz^3$ does (i.e length
squared)\footnote{The length of a edge of course is simply given by,
  for example, $l_1 = \int \| \basis{1} \| \thinspace dz^1$. Here, the
  quantity $ \| \basis{1} \| \thinspace dz^1$ has the units of
  length.}.

\section{Finite-Volume Schemes}

Before considering the discontinuous Galerkin scheme, consider a
finite-volume approach to solve \eqr{\ref{eq:advect}} directly. For
this we will assume that we have divided the domain into hexahedra
with flat, quadrilateral, faces. Integrate over a single such hex,
$\Omega$, to get the weak-form
\begin{wrapfigure}{L}{0.25\textwidth}
\incfig{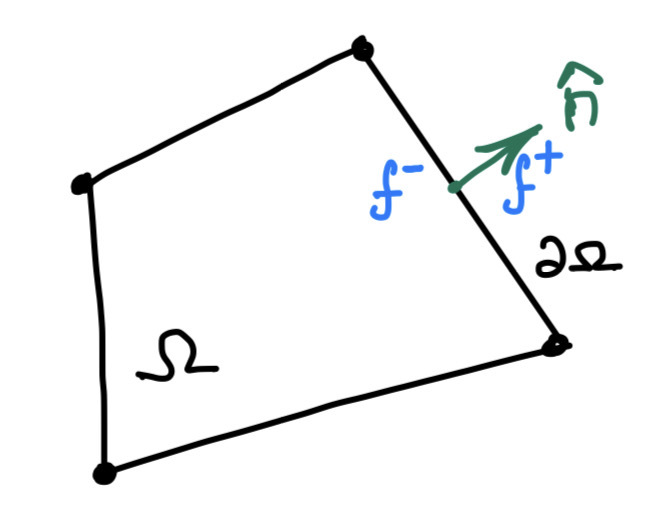} 
\caption{A hexahedral cell $\Omega$, with surface $\partial\Omega$ and
outward-pointing surface normal $\mvec{n}$.}
\label{fig:fv-cells}
\end{wrapfigure}
\begin{align}
  \frac{d}{dt} \int_\Omega f(\mvec{x},t) \thinspace d^3\mvec{x}
  +
  \oint_{\partial \Omega} \mvec{v}\cdot\mvec{n} \hat{f} \thinspace ds
  =
  0. \label{eq:fv-scheme-xs}
\end{align}
Here, $\mvec{n}$ is the unit normal vector on the faces
$\partial\Omega$ that bound the hex. (We have six such faces and the
$\oint$ is a short-hand for computing the integrals over each
individual face). The value $\mvec{v}\cdot\mvec{n} \hat{f}$ is the
\emph{numerical flux} on the face: this is computed using the values
of $f$ on each side of the face. See
Fig\thinspace(\ref{fig:fv-cells}).

This numerical flux can be computed from\footnote{This form of the
  flux is often called the ``Lax flux''. As written we are assuming
  the $\mvec{v}$ is a continuous vector field and hence we only have a
  single value of the normal component of the velocity at the face.}
\begin{align}
  \mvec{v}\cdot\mvec{n} \hat{f}
  =
  \mvec{v}\cdot\mvec{n} \llbracket f \rrbracket
  -
  | \mvec{v}\cdot\mvec{n} | \{ f \}
\end{align}
where $\llbracket f \rrbracket = (f^+ + f^-)/2$ and
$\{ f \} = (f^+ - f^-)/2$. Note that this numerical flux is
\emph{consistent}, i.e. when $f^+ = f^- = f$ (where $f$ is the common
value) then the numerical flux is identical to the physical flux
$\mvec{v}\cdot\mvec{n} f$. This consistency condition is
\emph{critical to ensure we are actually solving the correct equations
  and getting the physics right}.

If we sum \eqr{\ref{eq:fv-scheme-xs}} over all hexahedra in the
domain, then as we have use a common flux value across each face, we
will get that the discrete finite-volume scheme conserves total
particles in the domain. Note an important point: conservation of
particles \emph{did not depend on using a consistent flux}, just a
\emph{common} flux across each face. Hence, \emph{flux consistency} is
an \emph{independent} property from conservation.

Now consider a finite-volume scheme derived from the
\emph{transformed} advection equation \eqr{\ref{eq:advect-cs}}. For
this, we multiply by $J_c$ and integrate over a single, rectangular,
\emph{computational space} cell $I_{ijk} =
[z^1_{i-1/2},z^1_{i+1/2}]\times [z^2_{j-1/2},z^2_{j+1/2}] \times [z^3_{k-1/2},z^3_{k+1/2}]$ to get
\begin{align}
  \frac{d}{dt} \iiint_{I_{ijk}} f J_c \thinspace dz^1 dz^2 dz^3
  +
  \iint_{S_{jk}}  J_c \dbasis{1}\cdot\mvec{v} \hat{f} \thinspace dz^2 dz^3
  \bigg |^{i+1/2}_{i-1/2}
  + \ldots
  =
  0. \label{eq:fv-scheme-cs}
\end{align}
Here, $S_{jk}$ is the $z^1 = \textrm{constant}$ face of cell
$I_{ijk}$. We have dropped the other surface terms from the $z^2$- and
$z^3$ directions, but they can be treated in the same way. In general,
this scheme is different than one obtained from
\eqr{\ref{eq:fv-scheme-xs}}.

However, comparing the two schemes we see a few key points. First, the
quantity $J_c dz^1 dz^2 dz^3$ that appears in the first term in
\eqr{\ref{eq:fv-scheme-cs}} is needed to compute the total number of
particles in the \emph{mapped} physical cell. Second, the $J_c$ that
appears in the surface terms must be chosen very carefully: when
combined with the dual vector into $J_c \dbasis{1} dz^2 dz^2$ it must
give the \emph{surface area} element on the $z^1 = \textrm{constant}$
surface. It must hence be the \emph{same} as used in computing the
surface area of the cell in physical space. Further, the value of
$J_c$ (and of course the $\dbasis{1}$ vector) must the same as
computed from the two cells that are attached to the $S_{jk}$
face. Hence, in a way, it is more accurate to write the surface term
as
\begin{align}
  \iint_{S_{jk}}  \hat{f} \mvec{v}\cdot \ndbasis{1}
  \thinspace ( J_c \| \dbasis{1} \| dz^2 dz^3 )
  \bigg |^{i+1/2}_{i-1/2}
\end{align}
where $\ndbasis{1}$ is the normalized dual vector which is, of course,
the unit normal to the $S_{jk}$ surface in physical space.  In this
form, the quantity $J_c \| \dbasis{1} \| dz^2 dz^3$ appears as the
purely geometric quantity with units of area. For use in the surface
term we can use Lax fluxes:
\begin{align}
  \mvec{v}\cdot \ndbasis{1} \hat{f}
  =
  \mvec{v}\cdot\ndbasis{1} \llbracket f \rrbracket
  -
  | \mvec{v}\cdot\ndbasis{1} | \{ f \}.
  \label{eq:lax-flux-cs}
\end{align}
As an implementation detail we mention that in most finite-volume
codes (like the \gke\ wave-propagation fluid solvers) we do not
actually work with $J_c$ or $J_c \| \dbasis{i} \|$ but instead replace
them with the \emph{ratio} of the physical to computational space
volume, and the \emph{ratio} of the physical to computational space
surface areas, respectively. In addition, we do not store $\basis{i}$
and $\dbasis{i}$ but instead store an \emph{orthonormal} set of
vectors $\mvec{n}, \gvec{\tau}_1, \gvec{\tau}_2$ (with
$\mvec{n} = \gvec{\tau}_1\times \gvec{\tau}_2$) on each face of the
grid\footnote{For solving scalar equations (like the advection
  equations) we only need to have the surface normal $\mvec{n}$. The
  tangent vectors are needed, however, when, for example, solving the
  momentum, electromagnetic field, or pressure tensor equations.}. We
call this approach a \emph{triad-first} approach. We have generalized
this into a \emph{tetrads-first} approach for use in
general-relativity.

\section{Discontinuous Galerkin Schemes}

To derive a DG scheme let $\mathcal{U}$ be a finite-dimensional
function space defined in each computational space cell
$I_{ijk}$. Then, a DG scheme is one for which, for all
$w \in \mathcal{U}$ we have
\begin{align}
  \iiint_{I_{ijk}} w \pfraca{t} (f J_c)_h \thinspace dz^1 dz^2 dz^3
  &+
  \iint_{S_{jk}}  w^{-} J_c \dbasis{1}\cdot\mvec{v} \hat{f} \thinspace dz^2 dz^3
  \bigg |^{i+1/2}_{i-1/2}
  + \ldots \notag \\
  &-
  \iiint_{I_{ijk}} \pfrac{w}{z^i} (\dbasis{i}\cdot\mvec{v})_h (f J_c)_h \thinspace dz^1 dz^2 dz^3
  =
  0. \label{eq:dg-scheme-cs}  
\end{align}
We have shown only a single surface term, but the other terms can be
treated identically. Note that the DG scheme determines the projection
$(f J_c)_h$ on basis functions and not $f_h$ directly\footnote{ We are
  using our standard notation here and use the $h$ subscript to
  indicate projection on the basis functions. When manipulating
  equations involving projections we need to be very careful not to
  mess up the \emph{values} of the integrals that appear in the volume
  term. If we are \emph{not} careful we will introduce aliasing errors
  into the scheme and these are troublesome for high-$k$
  modes. Unfortunately, some sort of aliasing is \emph{unavoidable} in
  the surface terms as they may be inherently \emph{nonlinear} even
  for linear problems.}.  A weak-form of the latter can be obtained by
solving the weak equality
\begin{align}
  (f J_c)_h \doteq f_h J_{ch}
\end{align}
where $J_{ch}$ is the projection of the Jacobian on the basis
functions, in terms of which the physical cell volume is given by
\begin{align}
  \mathcal{V}_{ijk} = \iiint_{I_{ijk}} J_{ch} \thinspace dz^1 dz^2 dz^3.
\end{align}
To compute the surface terms we again group it as we did in the
finite-volume case:
\begin{align}
  \iint_{S_{jk}} w^{-} \hat{f} \mvec{v}\cdot \ndbasis{1}
  \thinspace ( J_c \| \dbasis{1} \| dz^2 dz^3 )
  \bigg |^{i+1/2}_{i-1/2}
\end{align}
The numerical flux can be computed using Lax fluxes,
\eqr{\ref{eq:lax-flux-cs}}. However, in computing the surface integral
we must be careful and ensure that the
$J_c \| \dbasis{1} \| dz^2 dz^3$ that appears in it, when integrated
over the surface gives the surface area of the $S_{jk}$ face of the
$I_{ijk}$ cell in physical space:
\begin{align}
  \mathcal{S}_{jk}
  =
  \iint_{S_{jk}} J_c \| \dbasis{1} \| \thinspace dz^2 dz^3.
  \label{eq:surf-area-dg}
\end{align}

The source of aliasing error is now apparent: to compute the numerical
flux we need the \emph{value} of $f$ at a node, but we only have the
volume projection $(f J_c)_h$. One way to compute this quantity is to
evaluate $(f J_c)_h$ at the node and then divide out by the
\emph{value} of $J_c$ at that node, this being the same \emph{value}
we used in \eqr{\ref{eq:surf-area-dg}}. Note that this value is
\emph{not, and must not} be the evaluation of the volume expansion of
$J_{ch}$ at the surface node! As the expansions of the Jacobian in the
two cells that share a face may be \emph{discontinuous}, this would
lead, in general, to discontinuous surface values, and hence a
\emph{geometric inconsistent} flux across the face.

It is also clear now that what we need is are \emph{exact} surface
normals, $\ndbasis{i}$, at each face. This is very reminiscent of the
\emph{triad-first} approach we already use in \gke, except that now
instead of a single normal we need to store normals at \emph{each} of
the evaluation nodes on every face\footnote{We can get away with a
  single normal on each face if we assume that the face of each cell
  is \emph{flat}. However, even for the simplest trilinear local
  mapping this need not be the case: it is not easy to ensure that
  four coplanar points in computational space are mapped to four
  coplanar points in physical space. Hence, in general, we will need
  to store normals at all evaluation nodes.}. Of course, only normals
are needed to update scalar equations, but we will need the two
surface tangents also for other equations (for example, in updating
the momentum equation in the PKPM model). Hence, it is possible we
should just store the orthonormal set of vectors
$\mvec{n}, \gvec{\tau}_1, \gvec{\tau}_2$ at each evaluation node on
each face. (Perhaps we could have two different structures: one with
just $\mvec{n}$ and the other with all three vectors to save memory).

\section{Multiblock Geometric Consistency}
\label{sec:mblock_consistency}

\begin{figure}
  \incfig{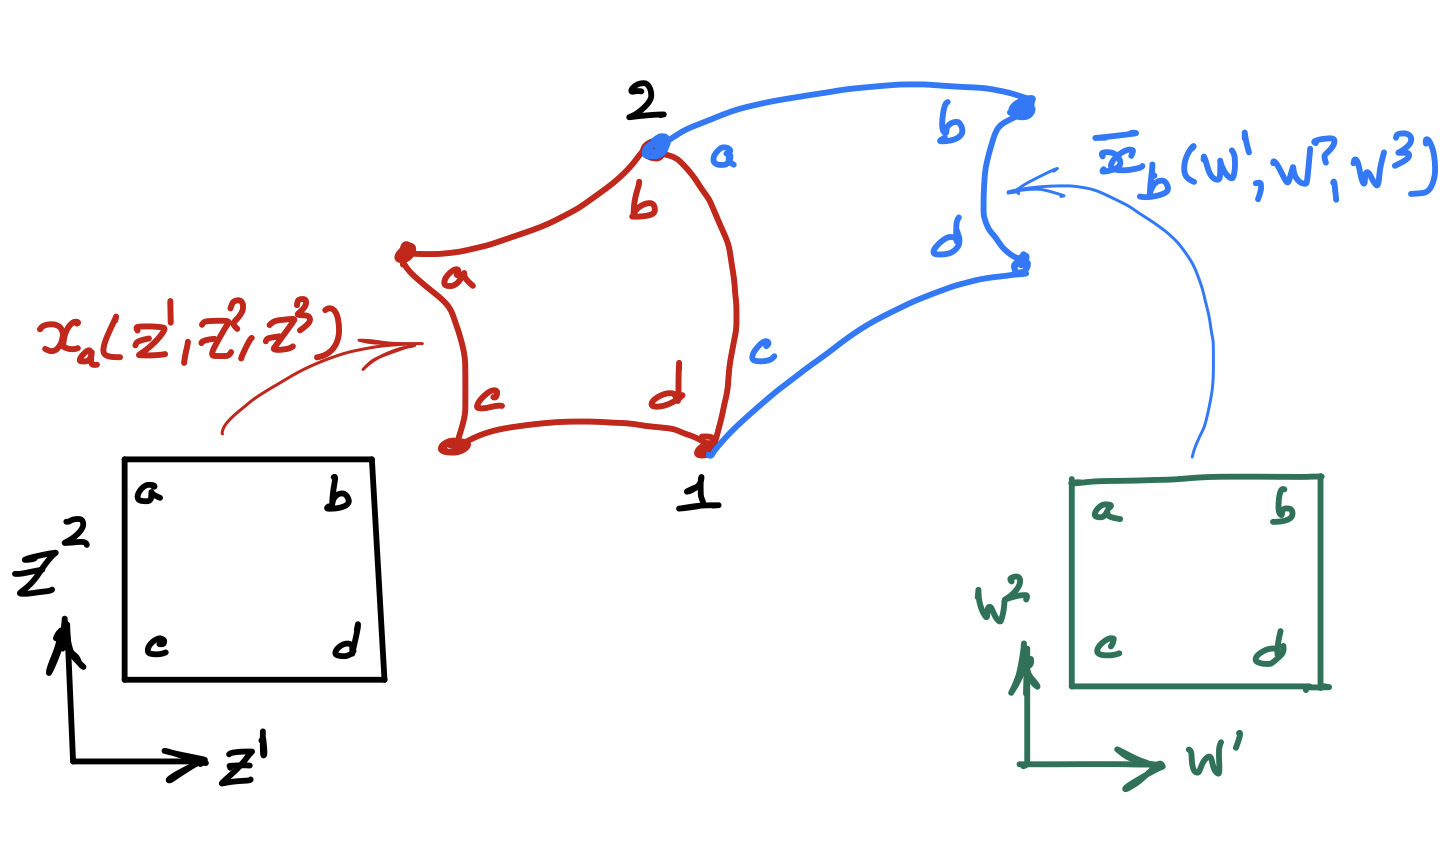}
  \setkeys{Gin}{width=0.75\linewidth,keepaspectratio}
  \caption{In this two-block case we have two mappings
    $\mvec{x}_a = \mvec{x}_a(z^1,z^2,z^3)$ and
    $\mvec{x}_b = \mvec{x}_b(w^1,w^2,w^3)$. These mappings must be
    \emph{consistent} at their shared surfaces: the normals computed
    from the two maps must be parallel and the tangent vectors on the
    common surface must span the same 2D space.}
  \label{fig:mbock}
\end{figure}

For many problems on complex geometry we need to use multiple patches
of coordinate mappings. see Fig.\thinspace\ref{fig:mbock}. Let us
assume we have two mappings
\begin{subequations}
\begin{align}
  \mvec{x}_a &= \mvec{x}_a(z^1,z^2,z^3) \\
\mvec{x}_b &= \mvec{x}_b(w^1,w^2,w^3).
\end{align}
\end{subequations}
From these we can compute the tangent vectors $\basis{i}$,
$\gbasis{g}{i}$ and their duals, $\dbasis{i}$, $\gdbasis{g}{i}$ in the
usual way.

Now consider the common face marked in the figure by the line
$(1,2)$. This is a $z^1 = \textrm{constant}$ and
$w^1 = \textrm{constant}$ surface. At this surface we have some
geometric consistency conditions. Let $\basis{2}$ and $\basis{3}$ be
the tangent vectors on this surface as computed using the $\mvec{x}_a$
mapping, and $\gbasis{g}{2}$ and $\gbasis{g}{3}$ be the tangent vectors
on this surface as computed using the $\mvec{x}_b$ mapping. Then we
must ensure that
\begin{align}
  \gbasis{g}{2}\cdot(\basis{2}\times\basis{3})
  =
  \gbasis{g}{3}\cdot(\basis{2}\times\basis{3})
  =
  0.
\end{align}
This merely states that the linear spaces spanned by
$(\basis{2},\basis{3})$ and $(\gbasis{g}{2}, \gbasis{g}{3})$ at each
point on the shared surface are the same. We must also have that
$\dbasis{1}\times\gdbasis{g}{1} = 0$. Further, as the surface is
shared, the surface area computed from either mapping must be the
same:
\begin{align}
  \mathcal{S}
  =
  \iint_1^2 J_{ca} \| \dbasis{1} \| \thinspace dz^2 dz^3
  =
  \iint_1^2 J_{cb} \| \gdbasis{g}{1} \| \thinspace dw^2 dw^3
  \label{eq:surf-match-mb}
\end{align}
where $J_{ca}$ and $J_{cb}$ are the Jacobians computed from the
$\mvec{x}_a$ and $\mvec{x}_b$ mappings respectively,

The geometric consistency is easier to impose on the tangent and dual
vectors than it is on the surface areas. The latter is particularly
tricky when doing DG schemes: we must ensure that the nodal points we
choose based on the $z^i$ and $w^i$ coordinates on shared surfaces
actually map to the \emph{same physical point} in physical space. This
need not need be the case as, in general, each of the two mappings may
be nonlinear and different. Further, we must ensure that the condition
\eqr{\ref{eq:surf-match-mb}} must be satisfied
\emph{exactly}. Otherwise we will introduce an error in particle flux
across block boundaries, potentially causing long-term instability in
the scheme.
